# Supplementary material for: Capacity: Cryptographically-Enforced In-Process Capabilities for Modern ARM Architectures (Extended Version)
Source: arXiv:2309.11151 source file (2023-09-20)
Supplement: Supplementary file 1 [file appendix.tex]

\newpage
\appendix

% \section{PARTS implementation details}
% \label{sec:parts}

% PARTS's instrumentation for \gls{dpi} is implemented in LLVM~\cite{llvm} 6.0.0 using its \emph{passes} infrastructure to perform program analysis and transformation. PARTS employs a pass that analyzes LLVM \emph{Intermediate Representation (IR)} to determines whether a LLVM load/store instruction contains a pointer in its operands, and encode the information in the instruction's \emph{metadata}. The metadata is then propagated from IR to \emph{machine IR (MIR)}, a representation that represents AArch64 assembly code, using a modified \emph{instruction selection} pass. The MIR metadata is then consumed by a \emph{machine pass}. In particular, on load and store instructions that access data pointers, the machine pass inserts instructions that move the pointers' SHA-3-generated type signature to a register to be used as \gls{pa}'s modifier, and inserts \texttt{pacda} \emph{before} a pointer is stored into memory for pointer signing, and \texttt{autda} \emph{after} a pointer is loaded from memory for authentication.

% % \thename proposes capability-based file-related reference authentication using \gls{pa}. As we already explained in ~\autoref{sec:design}, capability-based access control exhibits unique advantages in reference monitor designs for intra-process isolation; The need for a complicated bookkeeping of allowed file system resources and currently open file descriptors for each domain, is eliminated through non-forgeable references. 
\section{\thename's instrumented function}
\label{sec:asm}
\autoref{fig:asm-all} shows the instrumented listing in \autoref{fig:code-example} that we provided snippets of previously in \autoref{fig:asm}.
% \label{sec:asm}
% \begin{figure}[!h]
% \begin{lstlisting}[style=sslab-mini-c,language={[ARM]Assembler},linewidth=7.3cm,keepspaces]
% CAPAC_STACK  
% sensitive_func (CAPAC_VAR x0,  x1):
%  // INSTRUMENTED PROLOGUE
%  ...
%  // 1. Get current domain signature from
%  // DST[curr_dom]
%  ldr        dom_id, [curr_dom] 
%  ldr        dom_sig, [DST, dom_id]
%  // 2. Authenticate signature with domain key 
%  autdzb     dom_sig
%  cmp        dom_id, dom_sig 
%  b.ne       auth_failed
%  // Create a tag mask from domain id
%  lsl        tag_mask, dom_id, #56 
%  ... 
%  // 3. Tag stack and pointers
%  //  with  /*!\textcolor{clr-comment}{\textbf{T}$_{dom}$}!*/  /*!\hfill\action{Stack-Tag}!*/
%  subs       x20, sp, #16
%  mov        sp, x20
%  orr        x8, x20, x8                 
%  stg        x8, [x8]                   
%  ... 
%  // ON-STORE DOMAIN-AUTHENTICATED PTR SIGNING
%  // 1. Sign with domain key /*!\textcolor{clr-comment}{\key{DB}}!*/  /*!\hfill\action{PTR-Sign}!*/
%  pacdb      x0, modifier
%  // 2. Store pointer to memory 
%  str        x0, [x11]
%  ... 
%  // ON-STORE DOMAIN-AUTHENTICATED PTR AUTHENTICATION
%  // 1. Load pointer from memory
%  ldr         x0, [x11]                       
%  // 2. Authenticate with /*!\textcolor{clr-comment}{\key{DB}}!*/ /*!\hfill\action{PTR-Auth}!*/ 
%  autdb       x0, modifier                
%  ...
%  // ON-STORE AMBIENT PTR SIGNING
%  // 1. Tag is implicitly 0 (/*!\textcolor{clr-comment}{\textbf{T}$_{Amb}=0$}!*/) 
%  // 2. Sign with ambient key /*!\textcolor{clr-comment}{\key{DA}}!*/ 
%  pacda      x1, modifier /*!\hfill\action{PTR-Sign}!*/
%  // 3. Store pointer to memory 
%  str        x1, [sp, #20]
%  ...
%  // INSTRUMENTED EPILOGUE
%  // Untag and zero out the stack frame
%  stzg       sp, [sp]
%  add        sp, sp, #16
%  ...
%  ret
% \end{lstlisting}
% \caption{\thename's instrumentation for domain-authenticated pointers and stack memory isolation on an annotated function.}
% \label{fig:asm}
% % \vspace{-1em}
% \end{figure}

\begin{figure}[h]
\lstinputlisting[style=sslab-mini-c,language={[ARM]Assembler},linewidth=.9\columnwidth,keepspaces]{listings/instrumented.s}
\caption{\thename's instrumentation for domain-aware pointers authentication and stack memory isolation}
\label{fig:asm-all}
\end{figure}

\section{Algorithm for pointer liveness analysis}
\begin{algorithm}[t]
\tcc{Regs. \& frame indexes that contain ptrs.}
$P\gets\{\emptyset\}$\;
\tcc{Instr. that implicitly access ptrs. }
$S\gets\{\emptyset\}$\;
\For{Instruction $I$ in function}{
    \If{I.isStore()}{
        $accessPtr \gets false$\; 
        \If{$I.getSrc() \in R$}{
            $S \gets \{S \cup I\}$\;
            $accessPtr \gets true$\;
        } 
        \ElseIf{$I.accessPointer()$}{
            $S \gets \{S \cup I\}$\;
            $accessPtr \gets true$\;
        }
        \If{$I.isSpill()$}{
            \If{$accessPtr == true$}{
                $P \gets \{P \cup I.getDest()\}$
            }
            \lElse{$P \gets \{P - I.getDest()\}$}
        } 
    }
    \ElseIf{I.isLoad()}{
        $accessPtr \gets false$\; 
        \If{$I.getDest() \in P$}{
            $S \gets \{S \cup I\}$\;
            $accessPtr \gets true$\;
        } 
        \ElseIf{$I.accessPointer()$}{
            $S \gets \{S \cup I\}$\;
            $accessPtr \gets true$\;
        }
        \If{$accessPtr == true$}{
            $P \gets \{P \cup I.getSrc()\}$
        }
        \Else {$P \gets \{P - I.getSrc\}$}
    }
    $updateRegisterLiveness(I, R)$
}
\caption{Pointer liveness analysis}
\label{algo:liveness-analysis}
\end{algorithm}
\balance
